# Supplementary material for: Is BERT Blind? Exploring the Effect of Vision-and-Language Pretraining on Visual Language Understanding
Source: arXiv:2303.12513 source file (2023-11-02)
Supplement: Supplementary file 1 [file supp-probing.tex]

\subsection{Probing method details}

We present further implementation details of linear probing and Stroop probing, which we used for our tasks in addition to MLM probing.

\medskip \noindent \textbf{LP details}. 
For all linear probing tasks we used a logistic regression model using the scikit-learn \texttt{linear\_model.LogisticRegression} implementation. For all tasks we use the default parameters except for \texttt{max\_iter} which was changed according to task requirements. In particular, we used parameters \texttt{penalty='l2', C=1.0, solver='lbfgs'} for all tasks; \texttt{max\_iter} was set to 1,000 for the groundability task, 2,000 for linguistic acceptability and 400 for NLI.

\medskip \noindent \textbf{SP details}.
We proceed to describe the masked prompts used for Stroop probing as applied to the following tasks:

\begin{enumerate}
    \item{\textbf{Concreteness prediction}: We use the masked prompt \emph{"Alice giving a \MASK{} to Bob}"} and compare it to its completion when replacing the \MASK{} token with the various items tested. \\
    \item{\textbf{Color association prediction}: We use the sentence \emph{"A picture of a [OBJECT]"} as the masked probe, and compare it to the sentence \emph{"A picture of a [COLOR] [OBJECT]"}, where [COLOR] and [OBJECT] are replaced with the relevant color and object lexical items.}\\
    \item{\textbf{Geographical cloze test}: For the masked probe, we use the word \emph{'place'} in the position of the mask. This is compared to the probe with each possible answer inserted in the mask position.}\\
\end{enumerate}
