# Supplementary material for: Is BERT Blind? Exploring the Effect of Vision-and-Language Pretraining on Visual Language Understanding
Source: arXiv:2303.12513 source file (2023-11-02)
Supplement: Supplementary file 2 [file supp-cities.tex]

\section{Geographical cloze test details}

We treated all of the following as equivalent answers, since we saw that they are extremely frequent: 'u.s.', 'us', 'usa', 'u.s.a.' and 'u.s'

R@k metrics - micro-averaged (per question)
