# Supplementary material for: Is BERT Blind? Exploring the Effect of Vision-and-Language Pretraining on Visual Language Understanding
Source: arXiv:2303.12513 source file (2023-11-02)
Supplement: Supplementary file 3 [file supp-colors.tex]

\subsection{Color prediction }

We provide additional information regarding color prediction task. As different tokenizers have different lengths for same words, we only use samples with the following basic color labels which have single tokens for all models' tokenizers: [\emph{red, orange, yellow, green, blue, black, white, grey, brown}]. In particular, we did not use samples labelled as ``pink'' or ``purple'' since some models' tokenizers split these into multiple tokens, making it impossible to predict them from a single mask token with naive MLM.

Regarding the NCD dataset, for fruits and vegetables which have a strong association to more than one color, for example an apple which is associated with red and green, we allow both colors to be labeled as a valid prediction.
